# Supplementary material for: Improving Monocular Depth Estimation by Leveraging Structural Awareness and Complementary Datasets
Source: arXiv:2007.11256 source file (2020-07-22)
Supplement: Supplementary file 1 [file supplement_architecture.tex]

\begin{table}[t]
	\small
    \setlength{\tabcolsep}{3pt}
	\begin{center}
	\begin{tabular}{|c|c|c|c|c|c|c|c|}
		\hline
		\multicolumn{8}{|c|}{ \textbf{Encoder}} \\ \hline
		\multicolumn{2}{|c|}{ \textbf{Layer}} &\textbf{K} & \textbf{S} & \textbf{Channel} & \textbf{in} &\textbf{out}&\textbf{Input} \\ \hline
		\multirow{2}{*}{$\text{E}_1$}&$\text{conv}$ &7&2&3/64&H&H/2&\textbf{Input RGB}\\
		~&$\text{GCB}_1$&- &1&64/64&H/4&H/4	&$\text{conv}$ \\\hline
		\multirow{3}{*}{$\text{E}_2$}&maxpool & 3& 2 & 64/64& H/2& H/4& $\text{GCB}_1$ \\ 
		~&$\text{rblock}_1$ &1,3&1&64/256&H/4&H/4&$\text{maxpool}$ \\
		~&$\text{GCB}_2$&- &1&256/256&H/4&H/4	&$\text{rblock}_1$ \\\hline
		\multirow{2}{*}{$\text{E}_3$}&$\text{rblock}_2$ &1,3&2&256/512&H/4&H/8&$\text{GCB}_2$  \\
		~&$\text{GCB}_3$&-&1&512/512&H/8&H/8	&$\text{rblock}_2$ \\\hline
		\multirow{2}{*}{$\text{E}_4$}&$\text{rblock}_3$ &1,3&2&512/1024&H/8&H/16&$\text{GCB}_3$ \\ 
		~&$\text{GCB}_4$&-&1&1024/1024&H/16&H/16	&$\text{rblock}_3$ \\\hline
		\multirow{2}{*}{$\text{E}_5$}&$\text{rblock}_4$ &1,3&1&1024/2048&H/16&H/32&$\text{GCB}_4$ \\
		~&$\text{GCB}_5$&-&1&2048/2048&H/32&H/32	&$\text{rblock}_4$\\
		\hline
		\multicolumn{8}{|c|}{ \textbf{Decoder}} \\ \hline
		\multicolumn{2}{|c|}{ \textbf{Layer}} &\textbf{K} & \textbf{S} & \textbf{Channel} & \textbf{in} &\textbf{out}&\textbf{Input} \\ \hline
		\multirow{2}{*}{$\text{D}_5$} &$\text{upconv}_4$	&3	&2	&2048/1024&	H/32&	H/16&$\text{GCB}_5$	\\ 
		~&$\text{SAB}_4$&	1&	1&	2048/1024&	H/16&	H/16&	$\text{D}_5+\text{GCB}_4$  \\  \hline
		\multirow{3}{*}{$\text{D}_4$}&$\text{conv}_4$	&3&	1&	2048/1024&	H/16&	H/16&	$\text{SAB}_4$  \\
		~&$\text{upconv}_3$	&3&	2&	1024/512&	H/16&	H/8	&$\text{conv}_4$	\\ 
		~&$\text{SAB}_3$&	1&	1&	1024/512&	H/8&	H/8	&$\text{D}_4 +\text{GCB}_3$  \\ \hline
	    \multirow{3}{*}{$\text{D}_3$}& $\text{conv}_3$&	3&	1&	1024/512&	H/8&	H/8&	$\text{SAB}_3$   \\
		~&$\text{upconv}_2$	&3&	2&	512/256&	H/8&	H/4&	$\text{conv}_3$	   \\
		~&$\text{SAB}_2$&	1&	1&	512/256&	H/4&	H/4&$\text{D}_3 +\text{GCB}_2$   \\ \hline
		\multirow{3}{*}{$\text{D}_2$}&$\text{conv}_2$	&	3&	1&	512/256&	H/4&	H/4&	$\text{SAB}_2$  \\
		~&$\text{upconv}_1$&	3&	2&	256/64&	H/4	&H/2&	$\text{conv}_2$	   \\ 
		~&$\text{SAB}_1$&	1&	1&	128/64&	H/2&	H/2	&$\text{D}_2+\text{GCB}_1$   \\ \hline
	    $\text{D}_1$&$\text{conv}_1$		&3&	1&	64/64&	H/2	&H/2&  $\text{SAB}_1$  \\ \hline
	    
		\multicolumn{8}{|c|}{ \textbf{Output}} \\ \hline
		$\text{U}_4$&$\text{upshuffle}_3$&1&1 &1024/64&H/16&H &$\text{conv}_4$   \\ \hline
		$\text{U}_3$&$\text{upshuffle}_2$&1&1 &512/64 &H/8 &H &$\text{conv}_3$   \\ \hline
		$\text{U}_2$&$\text{upshuffle}_1$&1&1 &256/64 &H/4 &H &$\text{conv}_2$   \\ \hline
		$\text{U}_1$&$\text{upsample}_1$&-&-&128/64 &H/2 &H &$\text{conv}_1$   \\ \hline
		\multirow{2}{*}{Out}&$\text{conv}_0$	&3&	1&	256/128&	H&	H&$\text{U}_{1-4}$  \\
		~& \textbf{depth}&	3&	1&	64/1&	H&	H& $\text{conv}_0$	   \\
		\hline
	\end{tabular}
	\caption{The proposed network architecture. 
	    \textbf{K:}~kernel size, \textbf{S:}~stride in convolution layers,
	    \textbf{in} and \textbf{out:}~spatial resolution of the input and output, input: input of the layer.
		conv and conv:~convolution layer, upconv:~deconvolution layer.
		In the last column, + and $\text{U}_{1-4}$ denote concatenation for layers.
}
	\label{tab_architecture}
	\end{center}
\end{table}
