# Supplementary material for: Improving Monocular Depth Estimation by Leveraging Structural Awareness and Complementary Datasets
Source: arXiv:2007.11256 source file (2020-07-22)
Supplement: Supplementary file 2 [file supplement_architecture_new.tex]

\begin{table}%[t]
	\small
    \setlength{\tabcolsep}{8pt}
	\begin{center}
    \caption{Our proposed network architecture. \textbf{K}: kernel size; \textbf{S}: stride in convolution layers; \textbf{in} and \textbf{out}: spatial resolution of the input and output; \textbf{Input}: input of the layer. conv: convolution layer; upconv: upsample and convolution layer. In the last column, + and $\text{U}_{1-4}$ denote layer concatenation.}
	\begin{tabular}{|c|c|c|c|c|c|c|c|}
		\hline
		\multicolumn{2}{|c|}{ \textbf{Layer}} &\textbf{K} & \textbf{S} & \textbf{Channel} & \textbf{in} &\textbf{out}&\textbf{Input} \\ \hline
		\multicolumn{8}{|c|}{ \textbf{Encoder}} \\ \hline
		\multirow{2}{*}{$\text{E}_1$}&$\text{conv}$ &7&2&3/64&H&H/2&\textbf{input RGB}\\
		~&$\text{GCB}_1$&- &1&64/64&H/4&H/4	&$\text{conv}$ \\\hline
		\multirow{3}{*}{$\text{E}_2$}&maxpool & 3& 2 & 64/64& H/2& H/4& $\text{GCB}_1$ \\
		~&$\text{rblock}_1$ &1,3&1&64/256&H/4&H/4&$\text{maxpool}$ \\
		~&$\text{GCB}_2$&- &1&256/256&H/4&H/4	&$\text{rblock}_1$ \\\hline
		\multirow{2}{*}{$\text{E}_3$}&$\text{rblock}_2$ &1,3&2&256/512&H/4&H/8&$\text{GCB}_2$  \\
		~&$\text{GCB}_3$&-&1&512/512&H/8&H/8	&$\text{rblock}_2$ \\\hline
		\multirow{2}{*}{$\text{E}_4$}&$\text{rblock}_3$ &1,3&2&512/1024&H/8&H/16&$\text{GCB}_3$ \\
		~&$\text{GCB}_4$&-&1&1024/1024&H/16&H/16	&$\text{rblock}_3$ \\\hline
		\multirow{2}{*}{$\text{E}_5$}&$\text{rblock}_4$ &1,3&1&1024/2048&H/16&H/32&$\text{GCB}_4$ \\
		~&$\text{GCB}_5$&-&1&2048/2048&H/32&H/32	&$\text{rblock}_4$\\
		\hline
		\multicolumn{8}{|c|}{ \textbf{Decoder}} \\ \hline
%		\multicolumn{2}{|c|}{ \textbf{Layer}} &\textbf{K} & \textbf{S} & \textbf{Channel} & \textbf{in} &\textbf{out}&\textbf{Input} \\ \hline
		$\text{D}_5$ &$\text{upconv}_4$	&3	&2	&2048/1024&	H/32&	H/16&$\text{GCB}_5$	\\   \hline
		\multirow{3}{*}{$\text{D}_4$}&$\text{SAB}_4$&	1&	1&	2048/2048&	H/16&	H/16& $\text{D}_5+\text{GCB}_4$  \\
		~&$\text{conv}_4$	&3&	1&	2048/1024&	H/16&	H/16&	$\text{SAB}_4$  \\
		~&$\text{upconv}_3$	&3&	2&	1024/512&	H/16&	H/8	&$\text{conv}_4$	\\  \hline
		\multirow{3}{*}{$\text{D}_3$}&$\text{SAB}_3$&	1&	1&	1024/1024&	H/8&	H/8	&$\text{D}_4 +\text{GCB}_3$  \\
	    ~& $\text{conv}_3$&	3&	1&	1024/512&	H/8&	H/8&	$\text{SAB}_3$   \\
		~&$\text{upconv}_2$	&3&	2&	512/256&	H/8&	H/4&	$\text{conv}_3$	   \\ \hline
		\multirow{3}{*}{$\text{D}_2$}&$\text{SAB}_2$&	1&	1&	512/512&	H/4&	H/4&$\text{D}_3 +\text{GCB}_2$   \\
		~&$\text{conv}_2$	&	3&	1&	512/256&	H/4&	H/4&	$\text{SAB}_2$  \\
		~&$\text{upconv}_1$&	3&	2&	256/64&	H/4	&H/2&	$\text{conv}_2$	   \\  \hline
		\multirow{2}{*}{$\text{D}_1$}&$\text{SAB}_1$&	1&	1&	128/128&	H/2&	H/2	&$\text{D}_2+\text{GCB}_1$   \\
	    ~&$\text{conv}_1$		&3&	1&	128/64&	H/2	&H/2&  $\text{SAB}_1$  \\ \hline
		\multicolumn{8}{|c|}{ \textbf{Output}} \\ \hline
		\multirow{2}{*}{$\text{U}_4$}&$\text{conv}_5$	&3&	1&	1024/256&	H/16&	H/16&$\text{conv}_{4}$  \\
		~&$\text{upshuffle}_3$&-&- &256/1&H/16&H &$\text{conv}_5$   \\ \hline
		\multirow{2}{*}{$\text{U}_3$}&$\text{conv}_6$	&3&	1&	512/64&	H/8&	H/8&$\text{conv}_{3}$  \\
		~&$\text{upshuffle}_2$&-&- &64/1 &H/8 &H &$\text{conv}_6$   \\ \hline
		\multirow{2}{*}{$\text{U}_2$}&$\text{conv}_7$	&3&	1&	256/16&	H/4&	H/4&$\text{conv}_{2}$  \\
		~&$\text{upshuffle}_1$&-&- &16/1 &H/4 &H &$\text{conv}_7$   \\ \hline
		$\text{U}_1$&$\text{upsample}$&-&-&64/64 &H/2 &H &$\text{conv}_1$   \\ \hline
		\multirow{2}{*}{Out}&$\text{conv}_0$	&3&	1&	67/32&	H&	H&$\text{U}_{1-4}$  \\
		~& \textbf{depth}&	3&	1&	32/1&	H&	H& $\text{conv}_0$	   \\
		\hline
	\end{tabular}
	\label{tab_architecture}
	\end{center}
\end{table}
