# Supplementary material for: Improving Monocular Depth Estimation by Leveraging Structural Awareness and Complementary Datasets
Source: arXiv:2007.11256 source file (2020-07-22)
Supplement: Supplementary file 4 [file fig_supplement_false_edge.tex]

\begin{figure*}%[h]
	\includegraphics[width=\linewidth]{supplement_HC_false_edge.pdf}
	\caption{Qualitative results on the cases of \emph{spurious edges} from HC Depth dataset.}
	\label{fig_supplement_edge}
\end{figure*}
