# Supplementary material for: Improving Monocular Depth Estimation by Leveraging Structural Awareness and Complementary Datasets
Source: arXiv:2007.11256 source file (2020-07-22)
Supplement: Supplementary file 5 [file fig_supplement_nyu.tex]

\begin{figure*}
	\centering
	\includegraphics[width=\linewidth]{supplement_nyu}%
	\caption{Qualitative results on NYUDv2. From left to right: input images, ground-truth depth maps, Fu \etal~\cite{fu2018deep}, Hu \etal~\cite{hu2019revisiting}, Alhashim \etal~\cite{Alhashim2018}, our full model trained on NYUDv2, and our full model trained on all the six datasets. All the depth maps are visualized using the same scale.}
	\label{fig_supplement_nyu}
\end{figure*}
