# Supplementary material for: Improving Monocular Depth Estimation by Leveraging Structural Awareness and Complementary Datasets
Source: arXiv:2007.11256 source file (2020-07-22)
Supplement: Supplementary file 6 [file fig_supplement_nyu_cloud.tex]

\begin{figure*}
	\centering
	\includegraphics[width=\linewidth]{supplement_nyu_cloud.pdf}%
	\caption{Qualitative results on NYUDv2. From left to right, we show input images, depth maps visualized as point clouds using Fu \etal~\cite{fu2018deep}, Hu \etal~\cite{hu2019revisiting}, Alhashim \etal~\cite{Alhashim2018}, and our proposed method. The last column is the results of our full model trained on all the six datasets. The 3D point clouds of each example are rendered from the same viewpoint.}
	\label{fig_supplement_nyu_cloud}
\end{figure*}
